# Supplementary material for: Developing compact tuning fork thermometers for sub-mK temperatures and high magnetic fields
Source: arXiv:2107.02387 source file (2022-10-14)
Supplement: Supplementary file 2 [file Appendix.tex]

\appendix*
\clearpage
\section{}
\subsection{Preparation of the tuning forks}

The CTFs come in a vacuum tight can which must first be removed. Removing the vacuum can is typically accomplished by carefully crushing the fibreglass base until the tuning fork can be removed. Additionally, the leads that come soldered to the tuning fork are magnetic. For high field experiments, these leads must be removed and are replaced with contacts made using Electron Microscopy Sciences (EMS) 12642-14 silver epoxy. Afterwards, the CTF was mounted to a piece of stycast 1266-impregnated graph paper (stycast paper) The leads were glued to the paper with stycast to improve mechanical stability. The stycast paper was then attached to the polycarbonate insert for a \HeT cell shown in figure 1 in the main text and the leads soldered into the contact pins in the cell.

The array of tuning forks was patterned onto a quartz wafer of thickness $75~\si{\micro\meter}$. It was carefully removed from tabs on the wafer by scoring with a scribing tool and mounted on a piece of stycast paper. Contacts were made with EMS silver epoxy and the stycast paper mounted on the same cell insert as the CTF. During testing in room temperature air we established that the highest frequency tuning fork on this array showed the strongest resonant response, and therefore decided to focus on this tuning fork in the measurements presented here. This tuning fork is hereafter referred to as ATF5.

The cell insert was mounted in a \HeT cell in the experimental space of the Bay 3 cryostat at the NHMFL High B/T Facility. This cryostat is equipped with a PrNi$_5$/Cu nuclear demagnetisation stage precooled by a dilution refrigerator and a high field superconducting magnet capable of reaching temperatures of $1~\si{\milli\kelvin}$ and magnetic fields of $16~\si{\tesla}$ simultaneously. The cell itself was attached to the end of a silver cold finger that provides thermal contact to the demagnetisation stage. The \HeT in the cell condenses onto and is cooled by a sintered silver heat exchanger which is bolted to the cold finger. The tuning forks are immersed in the liquid \HeT and so their resonant properties provide a direct measurement of the viscosity, and hence the temperature of the \HeT. The cryostat is also equipped with a \HeT melting curve thermometer \cite{Ni1995}, which is mounted in the zero field space above the nuclear stage and provides an independent measurement of the cell temperature.
\subsection{Measurement Circuit}
\begin{figure}
\includegraphics[width=\columnwidth]{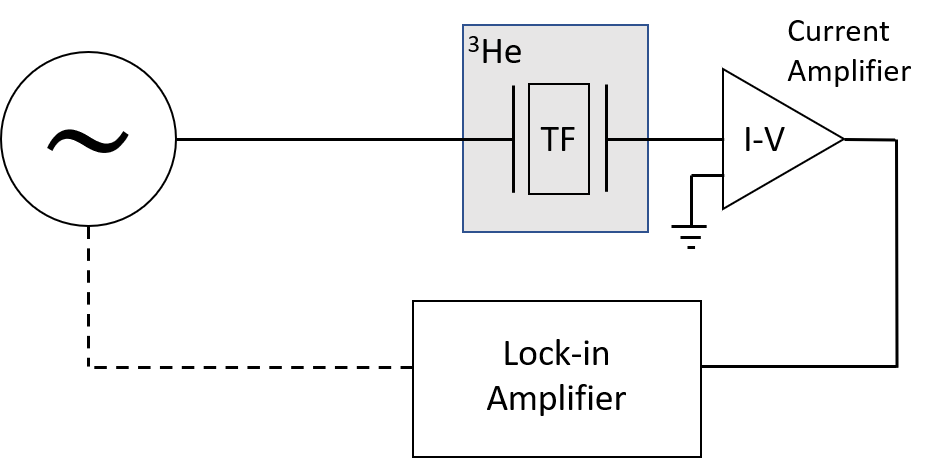}%
\caption{\label{forkCircuit}Schematic of the measurement setup for the tuning fork resonance curves. Shaded in grey is the low temperature, high magnetic field region where the tuning forks are immersed in liquid \HeT.}
\end{figure}
The tuning fork resonance curves were characterised using the setup shown in figure \ref{forkCircuit}. The AC driving voltage was supplied using a Keysight 33500B arbitrary waveform generator. Both sides of the tuning forks were connected to the inner conductor of coaxial leads, which were heat sunk at the various stages of the dilution refrigerator and finally at the nuclear stage. The outer conductors of the coaxial lines were connected together near the nuclear stage and grounded to the shared cryostat ground. The response current from the tuning fork was converted to a voltage using a home-built current to voltage converter~(gain $10^4$) and measured with a Stanford Research SR830 lock-in amplifier referenced to driving signal from the waveform generator.

\subsection{Mechanical properties of quartz tuning forks}
Tuning forks are piezoelectric resonators whose motion is driven by an AC voltage $V = V_0e^{i\omega{t}}$ with frequency $\omega$, which induces deflection of the tines via the piezoelectric effect. The stress caused by this deflection induces a current, which is maximum when the frequency of the driving signal matches the resonant frequency of the tines. 
The force on the tuning fork tines is given by
\begin{equation}
F = \frac{aV}{2},
\label{TFForce}
\end{equation}
where $a$ is the tuning fork constant. The response current is:
\begin{equation}
I = av,
\label{TFVel}
\end{equation}
where $v$ is the velocity of the tips of the tuning fork tines. Theoretically, the tuning fork constant $a$ depends on the dimensions of the tuning fork and the material properties of the quartz, it is given by \cite{Blaauwgeers2007}:
\begin{equation}
a = 3d_{11}E\frac{\mathcal{TW}}{\mathcal{L}},
\label{ForkConstTheory}
\end{equation}
where $d_{11}$ is the longitudinal piezoelectric modulus of quartz, $E$ is the Young's modulus and $\mathcal{T,W}$ and $\mathcal{L}$ are the dimensions of the tuning fork tines (figure 1 in main text).

In practice, the tuning fork constant can be derived directly from the properties of the resonance of the tuning fork (see below), yielding
\begin{equation}
a = \sqrt{\frac{4{\pi}m_{e}I_0\Delta{f}}{V_0}},
\label{ForkConstCalc}
\end{equation}
where $I_0$ is the response current amplitude at resonance, $\Delta{f}$ is the width of the tuning fork resonance and $m_{e} = 0.25\rho_q\mathcal{LWT}$ is the effective mass of a tuning fork tine. $\rho_q = 2659~\si{\kilogram\per\metre\cubed}$ is the density of quartz. Typically, the tuning fork constant derived experimentally is around $30 \%$ of the theoretical value \cite{Blaauwgeers2007}.

The tuning fork resonance is characterised by sweeping the frequency of the driving signal through the resonance at constant driving amplitude. The in-phase component, $X$ of the response is given by the real part of equation \ref{LorentzLineshape}, where
\begin{equation}
X = \frac{Af^2\Delta{f}^2}{(f_0^2-f^2)^2+(f\Delta{f})^2},
\label{LorentzInPhase}
\end{equation}
and the out-of-phase component $Y$ is the imaginary part
\begin{equation}
Y = \frac{Af\Delta{f}(f_0^2-f^2)}{(f_0^2-f^2)^2+(f\Delta{f})^2},
\label{LorentzOutPhase}
\end{equation}
Due to the measurement circuit, the tuning fork resonance will also have a non zero phase $\theta$ and a frequency dependent background, typically of the form $BG = a_0 + a_1f$. We then fit the equation: 
\begin{equation}
v(f) = X\cos{\theta} + Y\sin{\theta} + (a_0 + a_1f)
\label{FitModel}
\end{equation}
to obtain the amplitude $A$, resonant frequency $f_0$, resonance width $\Delta{f}$, phase $\theta$ and background coefficients $a_0$ and $a_1$ of the tuning fork resonance. The in-phase and out-of-phase components during a typical frequency sweep in vacuum are shown in figure \ref{vacRes}.

\begin{figure}
\includegraphics[width=\columnwidth]{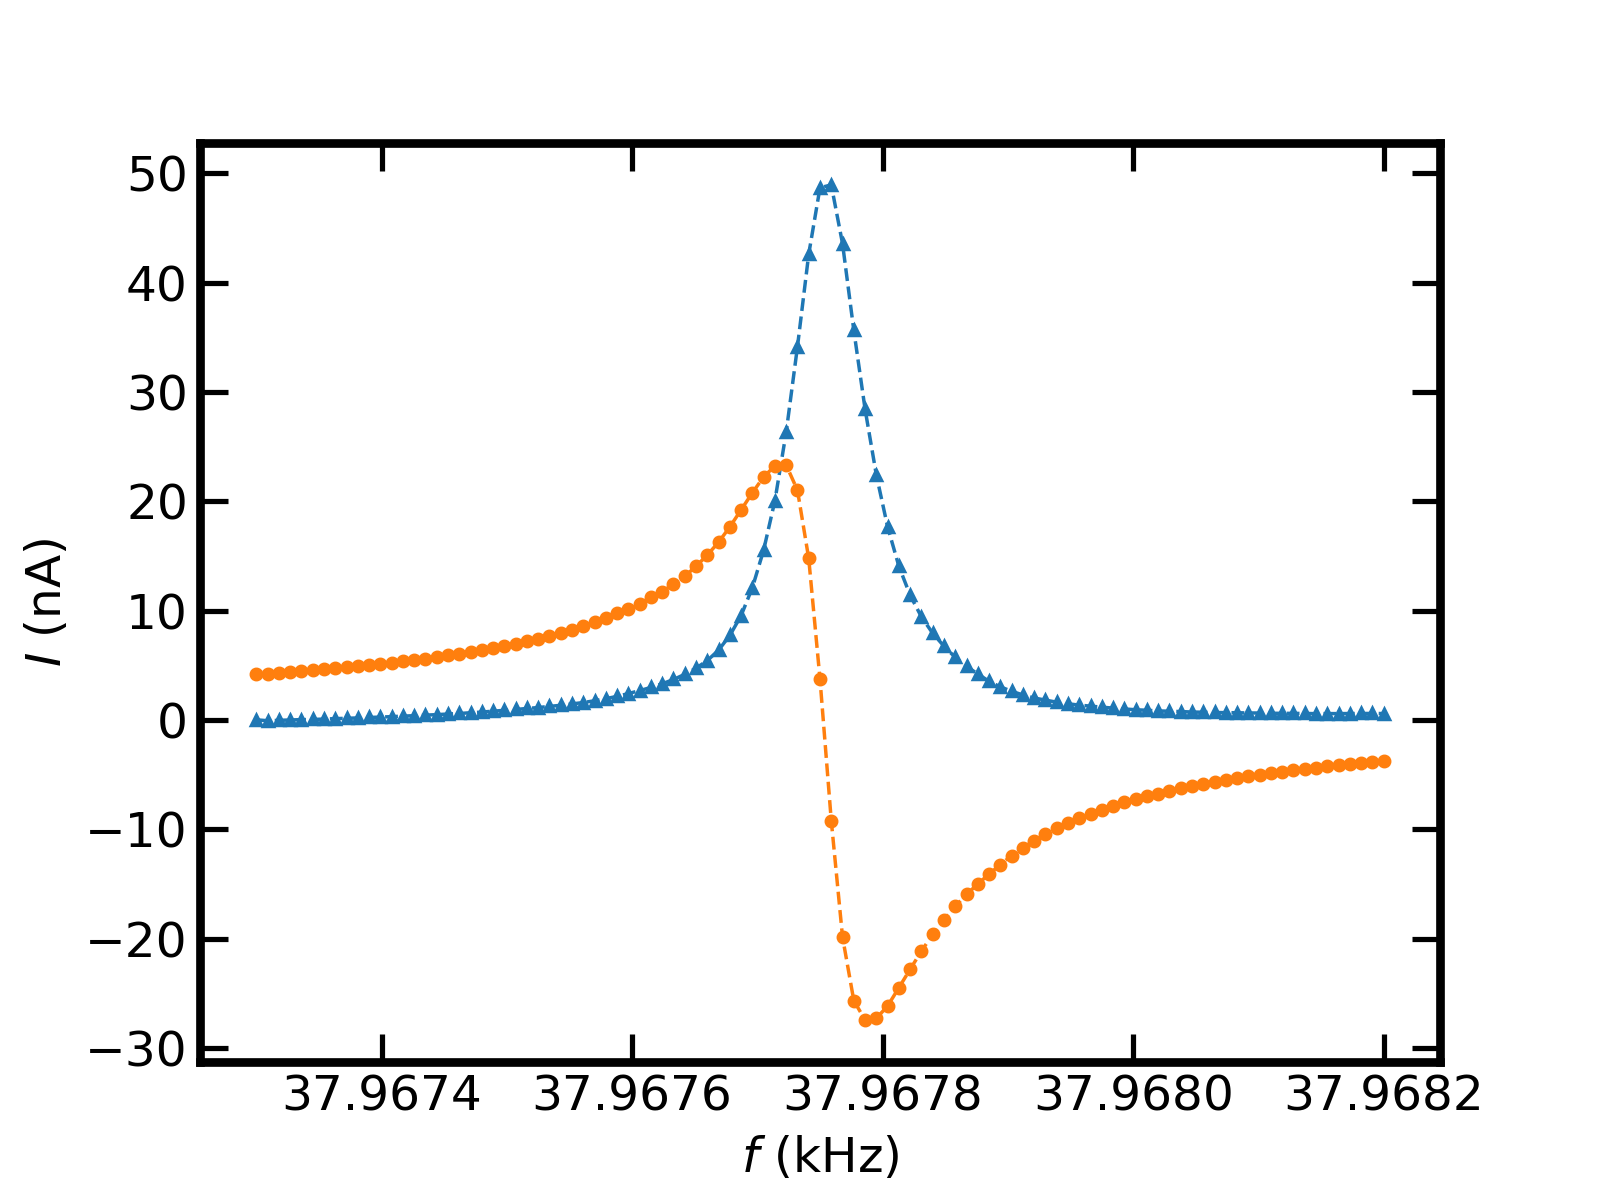}%
\caption{\label{vacRes}A typical frequency sweep obtained in vacuum on the array tuning fork at $T = 1 \si{\kelvin}$. The in-phase component is shown in blue and the out-of-phase in orange.}
\end{figure}

\subsection{Electromechanical model of the quartz tuning fork}
To describe the properties of the tuning fork resonance in fluid we model each tine as a damped harmonic oscillator with effective mass $m_{e}$ and spring constant $k$.

The equation of motion is
\begin{equation}
\frac{d^2u(t)}{dt^2} + \gamma\frac{du(t)}{dt} + \omega_0^2u(t) = \frac{F(t)}{m_{e}},
\label{AppEqMotion}
\end{equation}
where $u(t)$ is the displacement of the tip of the prongs, $\gamma$ describes the drag force, $F(t) = F_0e^{i\omega{t}}$ is the driving force and $\omega_0^2 = k/m_e$ is the vacuum resonance frequency. Modelling each prong as an ideal cantilever, the effective mass of the prong is:
\begin{equation}
m_e = 0.25\rho_q\mathcal{LWT}.
\label{AppEffMass}
\end{equation}
In a fluid, $\gamma$ has real and imaginary components, $\gamma = \gamma_2 + i\gamma_1$ where $\gamma_2$ describes dissipative drag forces while $\gamma_1$ describes the non-dissipative force arising from the fluid backflow.

Solving equation \ref{AppEqMotion} for the velocity $v = du/dt = v_0e^{iwt}$, where $u(t) = u_0e^(i\omega{t})$, of the tip of the tuning fork tine gives a velocity amplitude
\begin{equation}
v_0 = \frac{F_0}{m_e}\frac{\gamma_2\omega^2-i\omega(\omega_0^2-\omega^2-\omega\gamma_1)}{(\omega_0^2-\omega^2-\omega\gamma_1)^2+\gamma_2^2\omega^2}.
\label{LorentzLineshape}
\end{equation}
Assuming that $\gamma_1$ and $\gamma_2$ are constants much less than the resonant frequency, equation \ref{LorentzLineshape} describes a Lorentzian lineshape with width $\Delta{f} = \gamma_2/2\pi$.

At resonance, the tip velocity is maximum and has a value:
\begin{equation}
v_r = \frac{F_0}{2\pi{m_e}\Delta{f}}.
\label{maxVel}
\end{equation}
Using this along with equations \ref{TFForce} and \ref{TFVel} we can write the tuning fork constant:
\begin{equation}
a = \sqrt{\frac{4{\pi}m_{e}I_0\Delta{f}}{V_0}}.
\label{ForkConstCalcApp}
\end{equation}
